# Supplementary material for: RandOhm: Mitigating Impedance Side-channel Attacks using Randomized Circuit Configurations
Source: arXiv:2401.08925 source file (2024-08-30)
Supplement: Supplementary file 1 [file 08-Appendices.tex]

% \section*{Appendices}

% \appendix
% \subsection*{A. Validation Tests For Bit Extractions} \label{ApxA}
